# Supplementary material for: Temperature Dependence of Self-diffusion in Cr2O3 from First Principles
Source: arXiv:1904.04625 source file (2019-04-09)
Supplement: Supplementary file 1 [file SI_Cr2O3_HSE.pdf]

# Supporting Information to Temperature Dependence of Self-Diffusion in $Cr_2O_3$ from First Principles

Bharat Medasani,[*,†] Maria L. Sushko,[†] Kevin M. Rosso,[†] Daniel K. Schreiber,[‡] and Stephen M. Bruemmer[‡]

†*Physical and Computational Sciences Directorate*

‡*Energy and Environment Directorate, Pacific Northwest National Laboratory, Richland, WA 99354, USA*

E-mail: mbkumar@udel.edu,mbkumar@gmail.com

## Density Functional Calculations

We optimized $2 \times 2 \times 1$ supercells with the density functional theory (DFT) calculations using the Vienna *ab initio* simulation package (VASP).[1–3] HSE[4] hybrid functional with 25% mixing of Hartree Fock exchange at short range and a screening parameter of 0.6 was employed in conjunction with projector augmented wave (PAW) potentials[5,6] optimized for PBE[7] functional. Wave functions pre-optimized with PBEsol functional and GG+U method are used as input to the HSE calculations. A cut-off value of 400 eV was used for the plane-wave basis set and $2 \times 2 \times 1$ $\Gamma$-centered $k$-point grid was used to sample the reciprocal space. Spin polarization with anti-ferromagnetic (AFM) ordering of Cr spins was used. Gaussian method with a width of 0.01 eV was used for electronic smearing. The atomic positions in the defect supercells were relaxed at constant volume and fixed cell shape until the individual

forces on each atom were minimized to 0.03 eV/Å.

## Cr-O Phase Diagram

In generating the Cr-O phase diagram, elemental phases Cr and O, and compound phases $CrO_2$ and $Cr_2O_3$ are optimized with density functional theory (DFT). For all the phases, HSE functional with 25% short range mixing and a screening parameter of 0.6 was considered. Further, to maintain consistency with the defect calculations, the cells were relaxed with a plane wave basis set cutoff value of 400 eV. The total energies of the optimized phases were used to compute 0 K phase diagram given in Figure S1.

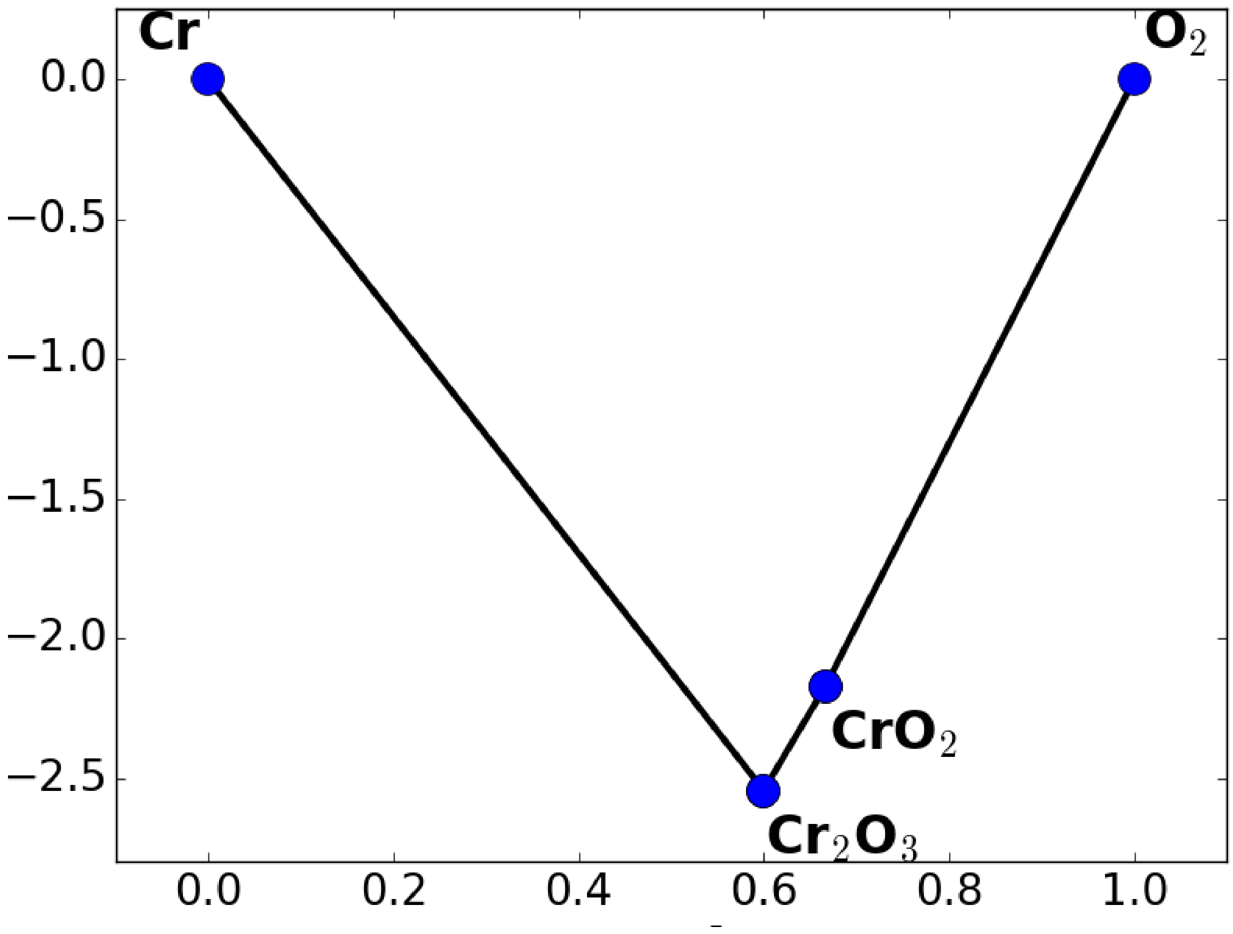


Figure S1: Cr-O phase diagram evaluated at O K. $x$-axis represents oxygen fractional composition. $y$-axis scale is eV/atom.

# Charge distribution of excess holes and electrons

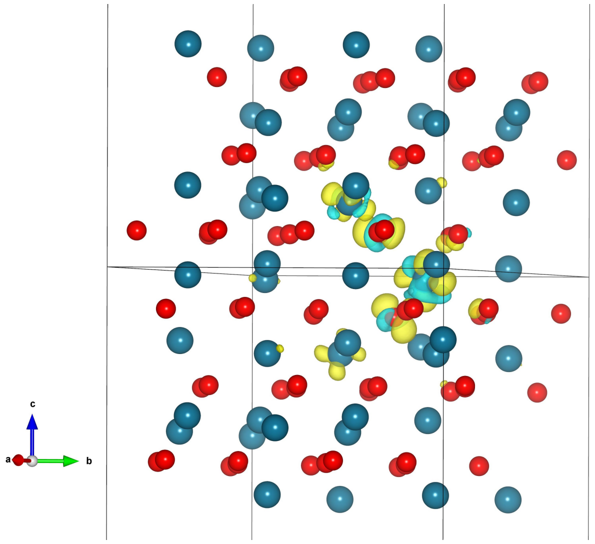


(a) $V_{Cr}^{-1}$

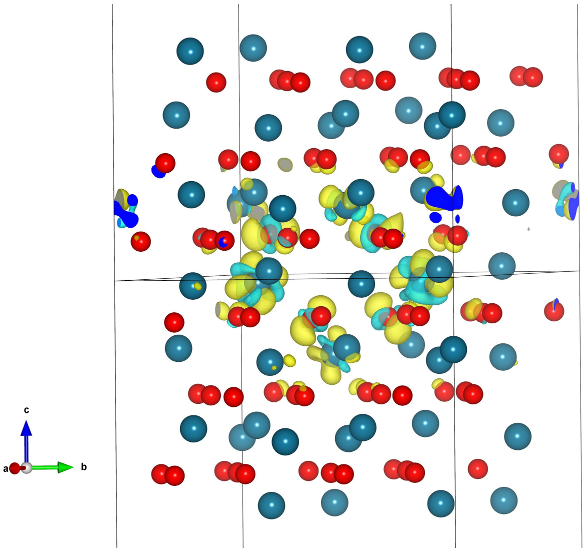


(b) $V_{Cr}^{-2}$

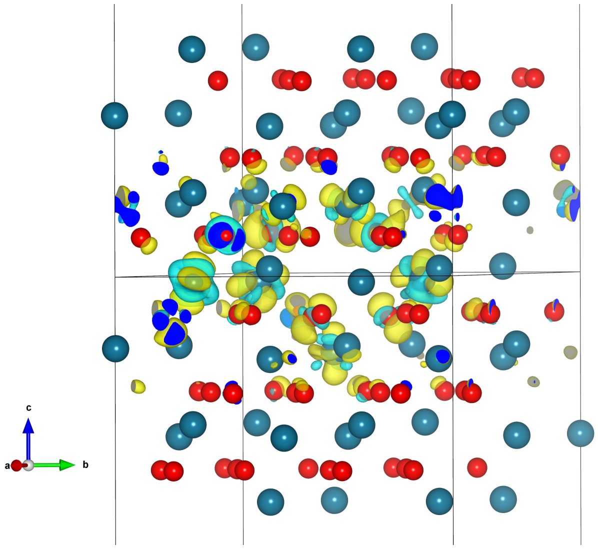


(c) $V_{Cr}^{-3}$

Figure S2: Distribution of excess electrons associated with charged Cr vacancies. The absolute magnitude of charge at yellow (-ve) and blue (+ve) iso-surfaces is 5 millielectrons/$\mathring{A}^3$.

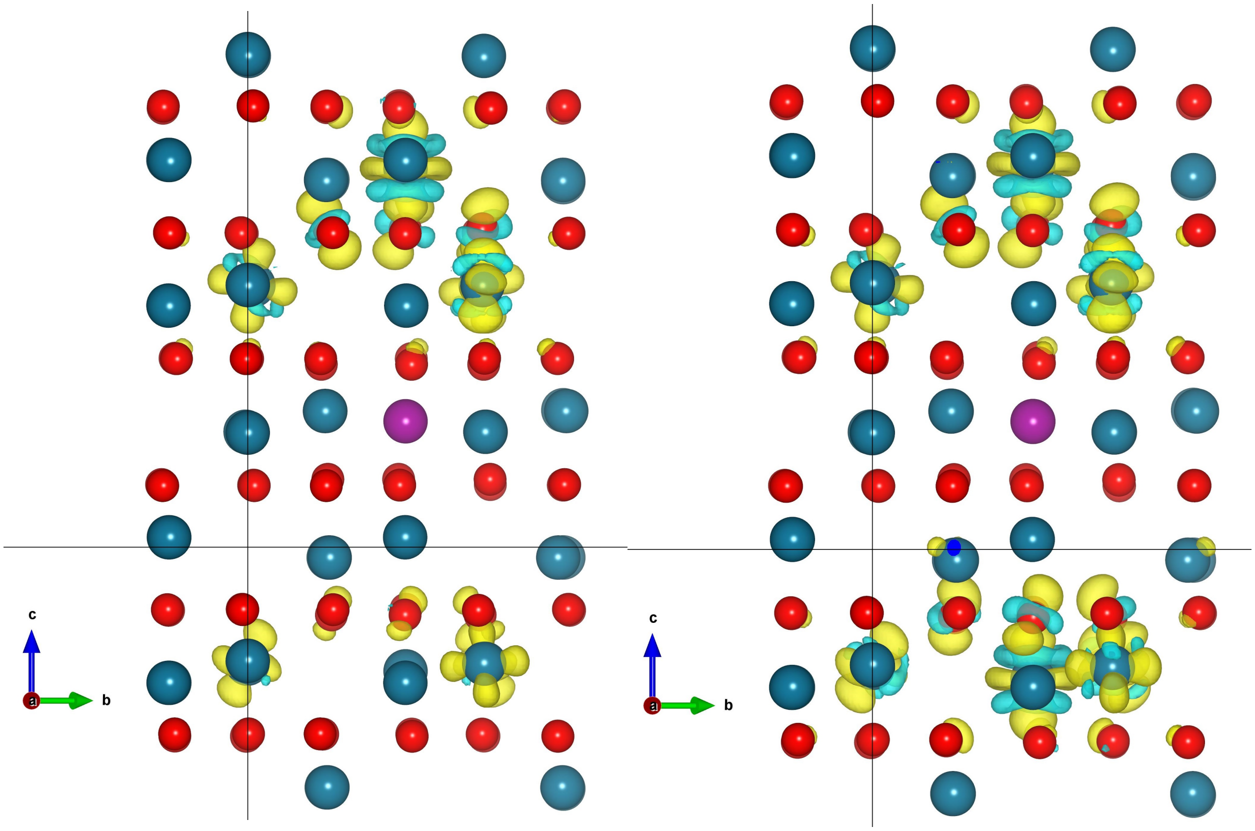


(a) $V_{Cr-TD}^{-2}$ (b) $V_{Cr-TD}^{-3}$

Figure S3: Distribution of excess electrons associated with charged Cr vacancy triple defects (or split vacancies).

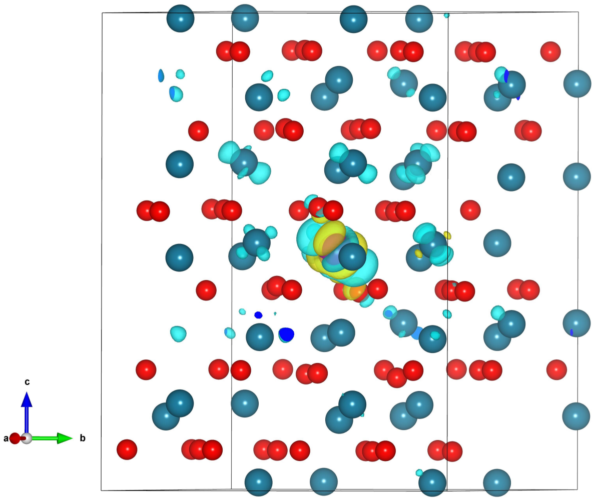

(a) $Cr_i^1$

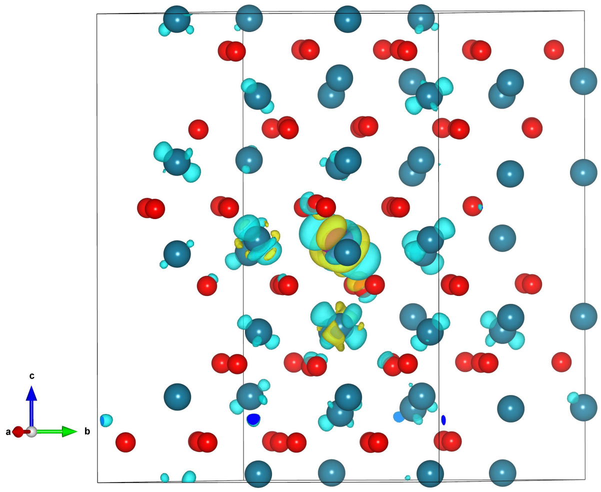

(b) $Cr_i^2$

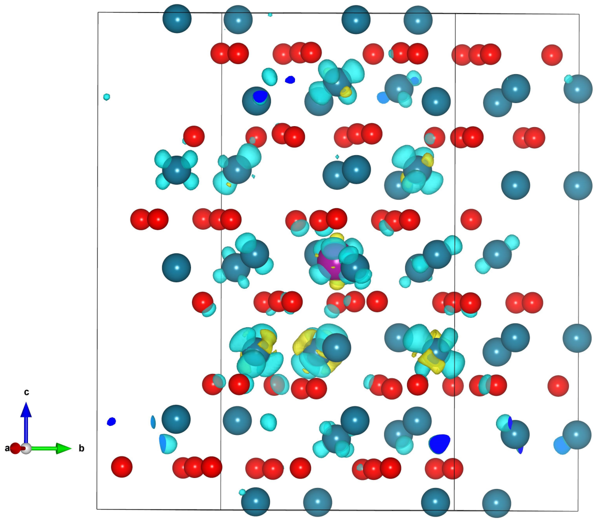

(c) $Cr_i^3$

Figure S4: Distribution of excess holes associated with charged Cr interstitials.

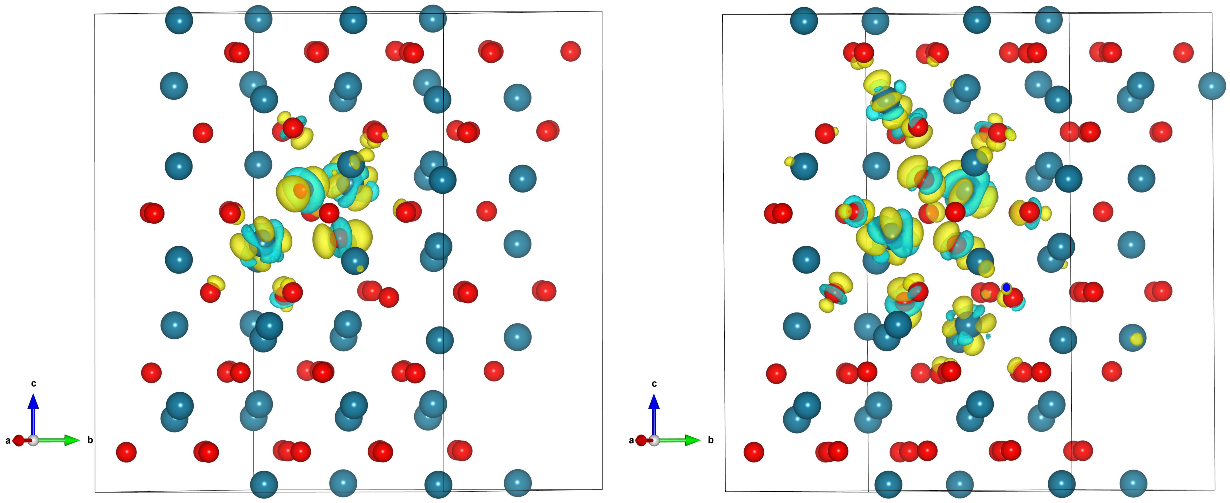

(a) $O_i^{-1}$ (b) $O_i^{-2}$

Figure S5: Distribution of excess electrons associated with charged O interstitials.

# 0-K Defect Formation Energies

## Anisotropic Electrostatic Corrections

The defect formation energies were corrected for spurious electrostatic interactions due to the periodic boundary conditions and the interaction of the defect with the compensating background charge. Electrostatic corrections were obtained with anisotropic FNV (Freysoldt, Neugebauer, and Vande Walle) method developed by Kumagai and Oba.[8,9] Table S2 lists the electrostatic corrections. In obtaining the corrections, experimentally reported dielectric tensor[10] was used.

Table S1: Electrostatic corrections to the defect formation energies of $Cr_2O_3$ obtained with HSE functional using anisotropic Freysoldt method.[8,9]

| Defect | q | Correction (eV) |
|---|---|---|
| $O_i$ | 0 | 0.000 |
| | -1 | 0.097 |
| | -2 | 0.447 |
| $Cr_i$ | 0 | 0.000 |
| | 1 | 0.284 |
| | 2 | 0.712 |
| | 3 | 1.443 |
| $V_O$ | 0 | 0.000 |
| | 1 | 0.188 |
| | 2 | 0.529 |
| $V_{Cr}$ | 0 | 0.000 |
| | -1 | 0.331 |
| | -2 | 0.958 |
| | -3 | 1.884 |
| $V_{Cr-TD}$ | 0 | 0.000 |
| | -1 | -0.123 |
| | -2 | -0.067 |
| | -3 | 0.230 |

Table S2: Defect transition levels with respect to valence band maximum.

| Defect | Charge Transition | Energy Level (eV) |
|---|---|---|
| $V_{Cr}$ | (-3, 0) | 2.032 |
| | (-3, -1) | 2.202 |
| | (-3, -2) | 2.373 |
| | (-2, 0) | 1.861 |
| | (-2, -1) | 2.032 |
| | (-1, 0) | 1.691 |
| $V_{Cr-TD}$ | (-3, 0) | 1.163 |
| | (-3, -1) | 1.291 |
| | (-3, -2) | 1.477 |
| | (-2, 0) | 1.008 |
| | (-2, -1) | 1.104 |
| | (-1, 0) | 0.912 |
| $Cr_i$ | (0, 1) | 3.737 |
| | (0, 2) | 3.567 |
| | (0, 3) | 3.242 |
| | (1, 2) | 3.396 |
| | (1, 3) | 2.996 |
| | (2, 3) | 2.602 |
| $V_O$ | (0, 1) | 1.600 |
| | (0, 2) | 1.360 |
| | (1, 2) | 1.120 |
| $O_i$ | (-2, 0) | 3.071 |
| | (-2, -1) | 2.655 |
| | (-1, 0) | 3.487 |

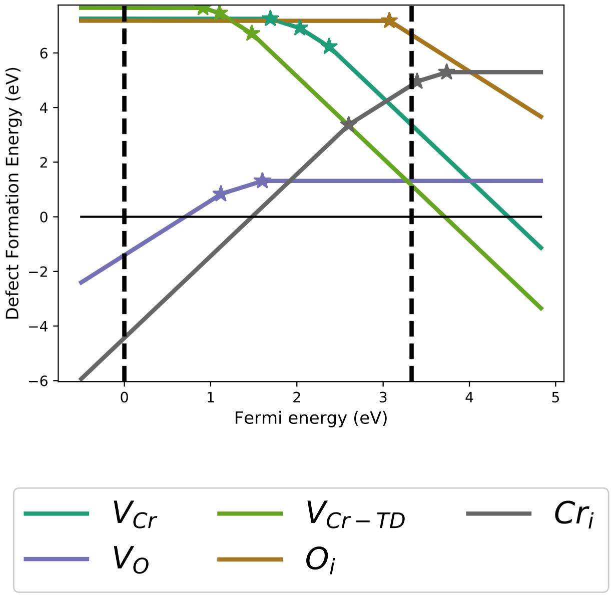


(a) Cr rich boundary

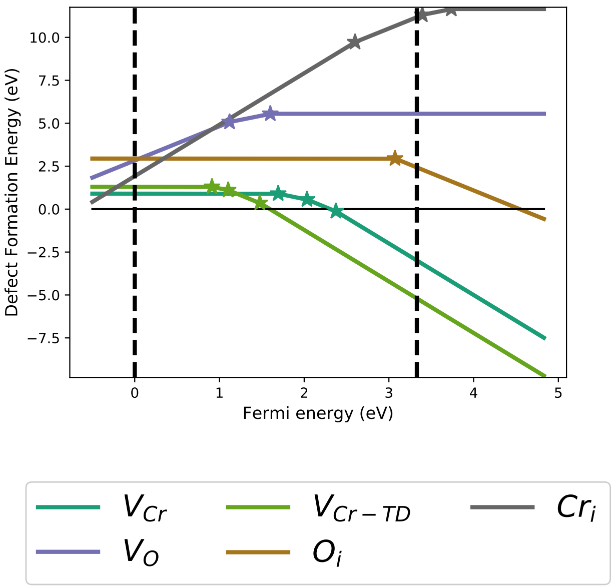


(b) O rich boundary

Figure S6: Formation energies of Cr and O interstitials at octahedral sites coordinated with 6 O atoms after accounting for electrostatic and bandgap related corrections. Black solid line corresponds to $E_f(Cr_i)$ and green dashed line refers to $E_f(O_i)$.

## References


(1) Kresse, G.; Hafner, J. *Phys. Rev. B* **1993**, *47*, 558–561.

(2) Kresse, G.; Hafner, J. *Phys. Rev. B* **1994**, *49*, 14251–14269.

(3) Kresse, G.; Furthmüller, J. *Phys. Rev. B* **1996**, *54*, 11169–11186.

(4) Heyd, J.; Scuseria, G. E.; Ernzerhof, M. *The Journal of Chemical Physics* **2003**, *118*, 8207–8215.

(5) Blöchl, P. E. *Phys. Rev. B* **1994**, *50*, 17953–17979.

(6) Kresse, G.; Joubert, D. *Phys. Rev. B* **1999**, *59*, 1758–1775.

(7) Perdew, J. P.; Burke, K.; Ernzerhof, M. *Phys. Rev. Lett.* **1996**, *77*, 3865–3868.

(8) Kumagai, Y.; Oba, F. *Phys. Rev. B* **2014**, *89*, 195205.

(9) Freysoldt, C.; Neugebauer, J.; Van de Walle, C. G. *Phys. Rev. Lett.* **2009**, *102*, 016402.

(10) Madelung, O., Rössler, U., Schulz, M., Eds. *Non-Tetrahedrally Bonded Binary Compounds II*; Springer Berlin Heidelberg: Berlin, Heidelberg, 2000; pp 1–6.
